# Supplementary material for: LiFT: Unsupervised Reinforcement Learning with Foundation Models as Teachers
Source: arXiv:2312.08958 source file (2023-12-14)
Supplement: Supplementary file 1 [file human.tex]

\begin{center}
\begin{tabular}{c | c}
    \toprule
       training environment indices & human-annotated task description \\ 
    \midrule
    
1 $\sim$ 5
& get milk from a cow
\\

6 $\sim$ 10
& shear a sheep and get some wool
\\

11 $\sim$ 15
& hunt a chicken and get its meat
\\

16 $\sim$ 20
& collect logs
\\

21 $\sim$ 25
& kill a cow
\\

26 $\sim$ 30
& kill a sheep
\\

31 $\sim$ 35
& kill a spider
\\

36 $\sim$ 40
& kill a zombie
\\

    \toprule
\end{tabular}
\label{tab:human}
\end{center}
